# Supplementary material for: CoHear: Conversation Enhancement via Multi-Earphone Collaboration
Source: arXiv:2505.21004 source file (2025-12-03)
Supplement: Supplementary file 1 [file appendix.tex]

\section{Data set matching algorithm}
\label{appendix:A}
We interpret the problem as a data set matching, which supposes the relative acoustic source positions as the vertices of a rigid body. Matching the rigid body shapes as observed by the different sensor nodes will result in an efficient way for geometry calibration as described in \cite{hennecke2009hierarchical}. In the following, we briefly recapitulate the concept of efficient geometry calibration based on data set matching \cite{gburrek2021geometry, sachar2004microphone}. 

Suppose for \(S_{k,l}\) refers to the relative locations of k sources in the coordinate system of the l sensor node,
\[
S_{k,l} = d_{k,l} [cos(\theta_{k,l}), sin(\theta_{k,l})]
\], where \(\theta_{k,l}\) and \(d_{k,l}\), corresponding to the azimuth and distance estimations. For each sensor node, we have rotation matrix \(R_{l}\) and translation vector \(n_{l}\), so we rewrite the relative locations of the \(k^{th}\) source in the global coordinates:
\[
S_{k} = R_{l} d_{k,l} [cos(\theta_{k,l}), sin(\theta_{k,l})] + n_{l}
\]
Ideally, multiple nodes observe each source at the same location in the global coordinate. As a result, we use only one subscription to differentiate it from \(S_{k,l}\).
Hence, the geometry can be inferred by minimizing the deviation of the projected source positions by the cost function below:
\[
\arg\min \sum_{l=1}^{L} \sum_{k=1}^{K} \left\| S_{k} - (R_{l} S_{k,l} + n_{l}) \right\|_2^2
\]
, where \( \| \cdot \|_2 \) denoting the Euclidean norm. There exists no closed-form solution for the above nonlinear optimization problem, so it has to be solved using an iterative optimization algorithm.

Let
\(
S^l = \begin{bmatrix} s_{0, l} \cdots & s_{K,l} \end{bmatrix}
\) be the matrix of all \( K \) source positions, as measured in the local coordinate system of sensor node \( l \). Similarly, let \( S \) be the same matrix of source positions but now measured in the global coordinate system. The dispersion matrix \( D_l \) is defined as follows \cite{35}:
\[
D_l = \frac{1}{K} (S^l - \overline{s}^l 1^T) W_l ( S - \overline{s} 1^T),
\]
where \( 1 \) denotes a vector of all ones. \( W_l \) is a diagonal matrix with \( W_{l,k,k} = w_{kl} \), where \( i,j \) denotes the \( i \)-th row and \( j \)-th column element of a matrix. \( \overline{s}^l \) corresponds to the centroid of the observations made by sensor node \( l \), and \( \overline{s} \) is the centroid of the source positions expressed in the global coordinate system:
\(
s^l = \frac{\sum_{k=1}^{K} w_{kl} s_{k,l}}{\sum_{k=1}^{K} w_{kl}}
\) 
and 
\(
\overline{s} = \frac{\sum_{k=1}^{K} w_{kl} s_k}{\sum_{k=1}^{K} w_{kl}}
\). The weights \( w_{kl} \) will be introduced later to control the impact of an individual observation \( s^l_k \) on the geometry estimates.

Carrying out a singular value decomposition (SVD) of the dispersion matrix gives \( D_l = U\sum V^T \). The estimate \( R_l \) of the rotation matrix is then given by \cite{sachar2004microphone}: \(\hat{R}_l = V U^T\), and the orientation of the corresponding sensor node by:
\(
\hat{\theta}_l = \text{arctan2}((\hat{R}_l)_{1,1}, \hat{R}_l)_{2,1}).
\)
Here, \text{arctan2} is the four-quadrant arc tangent. Thus, the \( l \)-th sensor node position estimate \( n_l \) in the reference coordinate system is given by
\(\hat{n}_l = \overline{n} - \hat{R}_l \overline{S}^l.
\)
Note that the described data set matching procedure is supposed to be applied to each sensor node.

Moreover, we consider the source positions as additional unknowns. The resulting cost function is optimized by alternating between the estimation of the set of source positions \( S \) and the estimation of the sensor node parameters \( S_{geo} = [R, n] \).
Starting from an initial set of source positions, the geometry can be determined for each sensor node \( l = 1, \ldots, L \) by data set matching, as outlined before. 
Given a geometry, the positions \( s_k \) can be estimated for each acoustic source \( k = 1, \ldots, K \) via:
\[
s_k = \arg\min_{s_k} \sum_{l=1}^{L} w_{kl} \| s_k - (R_{l} s_{k,l} + n_{l}) \|_2^2 \tag{14}
\]
For this, a closed-form solution exists, which is given by
\(s_k = \frac{\sum_{l=1}^{L} w_{kl} (R_{l} s_{k,l} + n_{l})}{\sum_{l=1}^{L} w_{kl}}\). What remains is to describe how the weights \( w_{kl} \) are chosen. They should reflect how well the observations \( s_{l}^{k} \) fit to the model specified by \( \text{geo} \) and \( s \). For example, this can be achieved by setting
\(w_{kl} = \frac{1}{\| s_k - (R_{l} s_{k,l} + n_{l}) \|_2^2} \).
